# Supplementary material for: CRUDE: Calibrating Regression Uncertainty Distributions Empirically
Source: arXiv:2005.12496 source file (2021-03-15)
Supplement: Supplementary file 1 [file appendix_table.tex]

% Please add the following required packages to your document preamble:
% \usepackage{booktabs}
% \usepackage{graphicx}
\begin{table*}[h]
\resizebox{\textwidth}{!}{%
\begin{tabular}{@{}lllllllllllllllll@{}}
\toprule
\multicolumn{1}{c}{} & \multicolumn{4}{c}{Variational NN Calibration}                                               & \multicolumn{4}{c}{Dropout NN Calibration}                                                    & \multicolumn{4}{c}{NGBoost Calibration}                                                       & \multicolumn{4}{c}{GP Calibration}                                                            \\ \midrule
\multicolumn{1}{c}{} & \multicolumn{1}{c}{-C} & \multicolumn{1}{c}{-C+S} & C              & \multicolumn{1}{c}{C+S} & \multicolumn{1}{c}{-C} & \multicolumn{1}{c}{-C+S} & C               & \multicolumn{1}{c}{C+S} & \multicolumn{1}{c}{-C} & \multicolumn{1}{c}{-C+S} & C               & \multicolumn{1}{c}{C+S} & \multicolumn{1}{c}{-C} & \multicolumn{1}{c}{-C+S} & C               & \multicolumn{1}{c}{C+S} \\ \midrule
fire                 & 0.106                  & 0.075                    & 0.069          & \textbf{0.061}          & 0.250                  & 0.069                    & 0.062           & \textbf{0.059}          & 0.227                  & 0.070                    & \textbf{0.057*} & 0.070                   & 0.388                  & 0.151                    & \textbf{0.082*} & 0.083                   \\
yacht                & 0.088                  & \textbf{0.084}           & 0.086          & 0.087                   & 0.186                  & \textbf{0.088}           & \textbf{0.088}  & 0.089                   & 0.099                  & 0.100                    & 0.097           & \textbf{0.094}          & 0.103                  & 0.071                    & \textbf{0.069}  & 0.079                   \\
auto                 & 0.091                  & 0.075                    & 0.076          & \textbf{0.063}          & 0.083                  & \textbf{0.072}           & 0.073           & 0.077                   & 0.073                  & 0.061                    & \textbf{0.060}  & 0.089                   & 0.096                  & 0.071                    & \textbf{0.069}  & 0.072                   \\
diabetes             & 0.079                  & 0.066                    & \textbf{0.063} & 0.073                   & 0.080                  & 0.063                    & \textbf{0.061}  & \textbf{0.061}          & 0.072                  & 0.071                    & \textbf{0.066}  & 0.072                   & 0.098                  & 0.076                    & \textbf{0.072}  & 0.074                   \\
housing              & 0.071                  & 0.062                    & \textbf{0.061} & 0.064                   & 0.093                  & 0.055                    & \textbf{0.053}  & 0.065                   & 0.104                  & 0.072                    & 0.070           & \textbf{0.066*}         & \textbf{0.055*}        & 0.058                    & \textbf{0.055}  & 0.063                   \\
energy               & 0.062                  & 0.056                    & \textbf{0.050} & \textbf{0.050}          & 0.073                  & 0.063                    & 0.051           & \textbf{0.045}          & 0.061                  & 0.058                    & 0.054           & \textbf{0.049}          & 0.061                  & 0.056                    & 0.055           & \textbf{0.046}          \\
concrete             & 0.048                  & 0.047                    & 0.046          & \textbf{0.034}          & 0.070                  & 0.061                    & 0.053           & \textbf{0.046}          & 0.056                  & 0.052                    & 0.052           & \textbf{0.049}          & 0.049                  & 0.043                    & 0.041           & \textbf{0.039}          \\
wine                 & 0.042                  & 0.033                    & 0.032          & \textbf{0.031}          & 0.056                  & 0.056                    & 0.037           & \textbf{0.032}          & 0.053                  & 0.046                    & 0.032           & \textbf{0.030}          & 0.052                  & 0.048                    & \textbf{0.032}  & 0.036                   \\
kin8nm               & 0.029                  & 0.017                    & \textbf{0.014} & 0.016                   & 0.032                  & 0.023                    & \textbf{0.018}  & 0.020                   & 0.054                  & 0.041                    & 0.017           & \textbf{0.016}          & 0.019                  & 0.018                    & 0.018           & \textbf{0.016}          \\
power                & 0.023                  & 0.017                    & 0.015          & \textbf{0.014}          & 0.023                  & 0.017                    & \textbf{0.015}  & 0.017                   & 0.016                  & 0.015*                   & \textbf{0.015}  & 0.017                   & 0.020                  & 0.013                    & \textbf{0.012}  & 0.013                   \\
airfoil              & 0.046                  & 0.042                    & \textbf{0.036} & 0.037                   & 0.055                  & 0.038                    & \textbf{0.033}  & 0.039                   & 0.047                  & 0.040                    & 0.039           & \textbf{0.037}          & 0.048                  & 0.043                    & 0.041           & \textbf{0.031}          \\
parkinsons           & 0.039                  & \textbf{0.019}           & \textbf{0.019} & \textbf{0.019}          & 0.042                  & 0.025                    & 0.022           & \textbf{0.020}          & 0.025                  & 0.022                    & \textbf{0.018}  & 0.019                   & 0.033                  & 0.019                    & 0.018           & \textbf{0.017}          \\ \midrule
                     & \multicolumn{4}{c}{Variational NN Calibration}                                               & \multicolumn{4}{c}{Dropout NN Calibration}                                                    & \multicolumn{4}{c}{NGBoost Calibration}                                                       & \multicolumn{4}{c}{Gaussian Process Calibration}                                              \\
                     & \multicolumn{1}{c}{-C} & \multicolumn{1}{c}{-C+S} & C              & \multicolumn{1}{c}{C+S} & \multicolumn{1}{c}{-C} & \multicolumn{1}{c}{-C+S} & C               & \multicolumn{1}{c}{C+S} & \multicolumn{1}{c}{-C} & \multicolumn{1}{c}{-C+S} & C               & \multicolumn{1}{c}{C+S} & \multicolumn{1}{c}{-C} & \multicolumn{1}{c}{-C+S} & C               & \multicolumn{1}{c}{C+S} \\ \midrule
fire                 & \textbf{3.435}         & 3.436                    & \textbf{3.435} & 3.533                   & \textbf{1.879}         & 1.881                    & \textbf{1.879*} & 2.317                   & \textbf{2.214}         & 2.218                    & \textbf{2.214}  & 2.623                   & \textbf{1.970}         & 2.021                    & \textbf{1.970}  & 2.971                   \\
yacht                & \textbf{0.128}         & \textbf{0.128}           & \textbf{0.128} & 0.130                   & 0.141                  & \textbf{0.140}           & 0.141           & 2.207                   & \textbf{0.062}         & \textbf{0.062}           & \textbf{0.062}  & 3.305                   & \textbf{0.124}         & \textbf{0.124}           & \textbf{0.124}  & 4.434                   \\
auto                 & \textbf{0.511}         & \textbf{0.511}           & \textbf{0.511} & 1.152                   & \textbf{0.382}         & \textbf{0.382}           & \textbf{0.382}  & 1.029                   & 0.512                  & \textbf{0.511}           & 0.512           & 1.706                   & \textbf{0.398}         & \textbf{0.398}           & \textbf{0.398}  & 0.975                   \\
diabetes             & 1.442                  & \textbf{1.441}           & 1.442          & 1.922                   & \textbf{0.843}         & \textbf{0.843}           & \textbf{0.843}  & 1.130                   & \textbf{1.027}         & \textbf{1.027}           & \textbf{1.027}  & 2.023                   & \textbf{0.870}         & \textbf{0.870}           & \textbf{0.870}  & 1.183                   \\
housing              & \textbf{0.467}         & \textbf{0.467}           & \textbf{0.467} & 0.742                   & 0.398                  & \textbf{0.397}           & 0.398           & 1.614                   & 0.486                  & \textbf{0.485}           & 0.486           & 1.625                   & 0.528                  & \textbf{0.527}           & 0.528           & 1.943                   \\
energy               & \textbf{0.138}         & \textbf{0.138}           & \textbf{0.138} & 0.538                   & \textbf{0.260}         & \textbf{0.260}           & \textbf{0.260}  & 0.624                   & \textbf{0.059}         & \textbf{0.059}           & \textbf{0.059}  & 2.047                   & \textbf{0.083}         & \textbf{0.083}           & \textbf{0.083}  & 1.624                   \\
concrete             & \textbf{0.407}         & \textbf{0.407}           & \textbf{0.407} & 0.814                   & 0.436                  & \textbf{0.435}           & 0.436           & 0.989                   & \textbf{0.355}         & \textbf{0.355}           & \textbf{0.355}  & 1.910                   & \textbf{0.505}         & \textbf{0.505}           & \textbf{0.505}  & 2.797                   \\
wine                 & \textbf{1.593}         & \textbf{1.593}           & \textbf{1.593} & 1.950                   & \textbf{0.935}         & \textbf{0.935}           & \textbf{0.935}  & 1.384                   & \textbf{0.941}         & \textbf{0.941}           & \textbf{0.941}  & 2.291                   & \textbf{1.067}         & \textbf{1.067}           & \textbf{1.067}  & 1.195                   \\
kin8nm               & \textbf{0.448}         & \textbf{0.448}           & \textbf{0.448} & 1.758                   & \textbf{0.401}         & \textbf{0.401}           & \textbf{0.401}  & 0.632                   & \textbf{0.653}         & \textbf{0.653}           & \textbf{0.653}  & 0.973                   & \textbf{0.333}         & \textbf{0.333}           & \textbf{0.333}  & 0.973                   \\
power                & \textbf{0.242}         & \textbf{0.242}           & \textbf{0.242} & 0.592                   & \textbf{0.283}         & \textbf{0.283}           & \textbf{0.283}  & 0.862                   & \textbf{0.236}         & \textbf{0.236}           & \textbf{0.236}  & 1.387                   & \textbf{1.347}         & 1.351                    & \textbf{1.347}  & 12.906                  \\
airfoil              & \textbf{0.509}         & \textbf{0.509}           & \textbf{0.509} & 2.503                   & 0.705                  & \textbf{0.703}           & 0.705           & 1.220                   & \textbf{0.411}         & \textbf{0.411}           & \textbf{0.411}  & 1.409                   & 0.539                  & \textbf{0.538}           & 0.539           & 1.081                   \\
parkinsons           & 0.114                  & \textbf{0.113}           & 0.114          & 0.396                   & \textbf{0.194}         & \textbf{0.194}           & \textbf{0.194}  & 1.926                   & \textbf{0.101}         & \textbf{0.101}           & \textbf{0.101}  & 1.499                   & \textbf{0.223}         & \textbf{0.223}           & \textbf{0.223}  & 2.233                   \\ \bottomrule
\end{tabular}%
}
\caption{Comparison of CRUDE, denoted C, with the negated version, denoted -C. +S denotes a learned shift factor. While CRUDE is consistently the best-calibrated, the learned shift with CRUDE substantially decreases its sharpness, unlike with the negated version. Moreover, we prefer the lack of shift for its theoretical simplicity.}
\label{shift-eval}
\end{table*}
